# Supplementary material for: Generalizable AI-Generated Image Detection Based on Fractal Self-Similarity in the Spectrum
Source: arXiv:2503.08484 source file (2026-08-19)
Supplement: Supplementary file 1 [file X_suppl.tex]

\clearpage
\setcounter{page}{1}
\maketitlesupplementary

\section{Comparison with More Methods}
\label{sec:rationale}
